# Supplementary material for: Efficient exposure computation by risk factor decomposition
Source: arXiv:1608.01197 ancillary file (2018-02-01)
Supplement: Supplementary file 1 [file YieldCurves_02122014.pdf]

EUR As of 2/12/2014

| Date       | Day  | Zero Rate  | Discount Factor |
|------------|------|------------|-----------------|
| 02/01/2015 | 31   | 0.0014886  | 0.99987         |
| 02/02/2015 | 62   | 0.00165636 | 0.99971869      |
| 02/03/2015 | 90   | 0.0017315  | 0.99957         |
| 02/04/2015 | 121  | 0.0017897  | 0.99941         |
| 04/05/2015 | 153  | 0.00181    | 0.99924         |
| 02/06/2015 | 182  | 0.0018039  | 0.9991          |
| 06/07/2015 | 216  | 0.001808   | 0.99893         |
| 04/08/2015 | 245  | 0.0018117  | 0.99878         |
| 04/09/2015 | 276  | 0.0018148  | 0.99863         |
| 05/10/2015 | 307  | 0.0018173  | 0.99847         |
| 04/11/2015 | 337  | 0.0018177  | 0.99832         |
| 04/12/2015 | 367  | 0.0018192  | 0.99817         |
| 04/01/2016 | 398  | 0.0018339  | 0.998           |
| 04/02/2016 | 429  | 0.0018518  | 0.99783         |
| 04/03/2016 | 458  | 0.0018668  | 0.99766         |
| 04/04/2016 | 489  | 0.0018877  | 0.99747         |
| 04/05/2016 | 519  | 0.0019088  | 0.99729         |
| 06/06/2016 | 552  | 0.0019295  | 0.99709         |
| 05/12/2016 | 734  | 0.0021235  | 0.99574         |
| 04/12/2017 | 1098 | 0.0026835  | 0.99196         |
| 04/12/2018 | 1463 | 0.0033846  | 0.98653         |
| 04/12/2019 | 1828 | 0.0042281  | 0.97905         |
| 04/12/2020 | 2194 | 0.0051937  | 0.96926         |
| 06/12/2021 | 2561 | 0.0062987  | 0.95677         |
| 05/12/2022 | 2925 | 0.0074624  | 0.94195         |
| 04/12/2023 | 3289 | 0.0086458  | 0.92505         |
| 04/12/2024 | 3655 | 0.0097639  | 0.90686         |
| 04/12/2025 | 4020 | 0.0107787  | 0.88806         |
| 04/12/2026 | 4385 | 0.0116748  | 0.86913         |
| 06/12/2027 | 4752 | 0.012493   | 0.84989         |
| 04/12/2028 | 5116 | 0.0131963  | 0.83113         |
| 04/12/2029 | 5481 | 0.013809   | 0.81272         |
| 04/12/2030 | 5846 | 0.0143494  | 0.79467         |
| 04/12/2031 | 6211 | 0.0148386  | 0.77686         |
| 04/12/2032 | 6579 | 0.0152614  | 0.75951         |
| 04/12/2033 | 6943 | 0.0156213  | 0.74294         |
| 04/12/2034 | 7307 | 0.015938   | 0.72683         |
| 04/12/2035 | 7672 | 0.0161984  | 0.71143         |
| 04/12/2036 | 8038 | 0.0164115  | 0.69669         |
| 04/12/2037 | 8403 | 0.0165929  | 0.68249         |
| 04/12/2038 | 8770 | 0.0167396  | 0.66884         |
| 04/12/2039 | 9134 | 0.0168765  | 0.65552         |
| 04/12/2040 | 9499 | 0.0169885  | 0.64267         |

USD As of 2/12/2014

| Date       | Day   |
|------------|-------|
| 02/01/2015 | 31    |
| 02/02/2015 | 62    |
| 02/03/2015 | 90    |
| 07/04/2015 | 126   |
| 05/05/2015 | 154   |
| 04/06/2015 | 184   |
| 17/06/2015 | 197   |
| 16/09/2015 | 288   |
| 16/12/2015 | 379   |
| 16/03/2016 | 470   |
| 15/06/2016 | 561   |
| 21/09/2016 | 659   |
| 05/12/2016 | 734   |
| 04/12/2017 | 1098  |
| 04/12/2018 | 1463  |
| 04/12/2019 | 1828  |
| 04/12/2020 | 2194  |
| 06/12/2021 | 2561  |
| 05/12/2022 | 2925  |
| 04/12/2023 | 3289  |
| 04/12/2024 | 3655  |
| 04/12/2026 | 4385  |
| 04/12/2029 | 5481  |
| 04/12/2034 | 7307  |
| 05/12/2039 | 9134  |
| 05/12/2044 | 10961 |
| 04/12/2054 | 14612 |
| 04/12/2064 | 18265 |

|            |       |           |         |
|------------|-------|-----------|---------|
| 04/12/2041 | 9864  | 0.0171046 | 0.62987 |
| 04/12/2042 | 10229 | 0.0171968 | 0.61759 |
| 04/12/2043 | 10594 | 0.0172778 | 0.60563 |
| 04/12/2044 | 10961 | 0.0173456 | 0.59399 |
| 06/12/2049 | 12788 | 0.0175937 | 0.53988 |
| 04/12/2054 | 14612 | 0.0177748 | 0.49087 |
| 04/12/2064 | 18265 | 0.0175409 | 0.41571 |

GBP As of 2/12/2014

| Zero Rate  | Discount Factor |            |       | Zero Rate | Discount Fact |
|------------|-----------------|------------|-------|-----------|---------------|
| 0.0024171  | 0.99979         | 02/01/2015 | 31    | 0.69638   | 0.99941       |
| 0.0024108  | 0.99959         | 02/02/2015 | 62    | 0.71036   | 0.99879       |
| 0.0023779  | 0.99941         | 02/03/2015 | 90    | 0.70235   | 0.99827       |
| 0.0024356  | 0.99916         | 02/04/2015 | 121   | 0.6987    | 0.99769       |
| 0.002464   | 0.99896         | 05/05/2015 | 154   | 0.69214   | 0.99708       |
| 0.0024879  | 0.99875         | 02/06/2015 | 182   | 0.67536   | 0.99664       |
| 0.0025143  | 0.99864         | 02/07/2015 | 212   | 0.69418   | 0.99598       |
| 0.00293409 | 0.99768756      | 03/08/2015 | 244   | 0.70916   | 0.99527       |
| 0.0035849  | 0.99628         | 02/09/2015 | 274   | 0.72002   | 0.99461       |
| 0.0044393  | 0.9943          | 02/10/2015 | 304   | 0.72873   | 0.99395       |
| 0.0053973  | 0.99174         | 02/11/2015 | 335   | 0.73611   | 0.99327       |
| 0.0064957  | 0.98834         | 02/12/2015 | 365   | 0.74075   | 0.99262       |
| 0.0073647  | 0.9853          | 02/06/2016 | 548   | 0.84374   | 0.98741       |
| 0.0114369  | 0.96618         | 02/12/2016 | 731   | 0.95998   | 0.98096       |
| 0.0147708  | 0.94251         | 04/12/2017 | 1098  | 1.18836   | 0.96488       |
| 0.0173264  | 0.91688         | 03/12/2018 | 1462  | 1.38277   | 0.94612       |
| 0.0193624  | 0.89013         | 02/12/2019 | 1826  | 1.54593   | 0.92558       |
| 0.021028   | 0.86283         | 02/12/2020 | 2192  | 1.68255   | 0.90389       |
| 0.0223908  | 0.83574         | 02/12/2021 | 2557  | 1.79745   | 0.88169       |
| 0.0235302  | 0.80894         | 02/12/2022 | 2922  | 1.90087   | 0.85884       |
| 0.0245184  | 0.7823          | 04/12/2023 | 3289  | 1.99145   | 0.83573       |
| 0.0261653  | 0.73027         | 02/12/2024 | 3653  | 2.07004   | 0.81288       |
| 0.0278846  | 0.65788         | 02/12/2026 | 4383  | 2.20688   | 0.7672        |
| 0.0295549  | 0.55341         | 03/12/2029 | 5480  | 2.35602   | 0.70207       |
| 0.0303151  | 0.46831         | 04/12/2034 | 7307  | 2.49703   | 0.6066        |
| 0.0306699  | 0.39811         | 02/12/2039 | 9131  | 2.54133   | 0.52954       |
| 0.0307061  | 0.29251         | 02/12/2044 | 10958 | 2.5598    | 0.46371       |
| 0.0300796  | 0.22197         | 02/12/2054 | 14610 | 2.52677   | 0.36371       |
|            |                 | 02/12/2064 | 18263 | 2.50931   | 0.28492       |



| JPY As of 2/12/2014 |            |                  |         |          |
|---------------------|------------|------------------|---------|----------|
| Discount Factor     | Day        | Number of D Rate |         | Discount |
|                     | 05/01/2015 | 34               | 0.10721 | 0.9999   |
|                     | 02/02/2015 | 62               | 0.10683 | 0.99982  |
|                     | 02/03/2015 | 90               | 0.10789 | 0.99973  |
|                     | 07/04/2015 | 126              | 0.1085  | 0.99963  |
|                     | 04/06/2015 | 184              | 0.10909 | 0.99945  |
|                     | 04/09/2015 | 276              | 0.11032 | 0.99917  |
|                     | 04/12/2015 | 367              | 0.11363 | 0.99886  |
|                     | 06/06/2016 | 552              | 0.11125 | 0.99832  |
|                     | 05/12/2016 | 734              | 0.10996 | 0.99779  |
|                     | 04/12/2017 | 1098             | 0.11991 | 0.9964   |
|                     | 04/12/2018 | 1463             | 0.14616 | 0.99416  |
|                     | 04/12/2019 | 1828             | 0.18755 | 0.99065  |
|                     | 04/12/2020 | 2194             | 0.23899 | 0.98574  |
|                     | 06/12/2021 | 2561             | 0.29956 | 0.9792   |
|                     | 05/12/2022 | 2925             | 0.36405 | 0.97125  |
|                     | 04/12/2023 | 3289             | 0.42878 | 0.9621   |
|                     | 04/12/2024 | 3655             | 0.49534 | 0.95161  |
|                     | 04/12/2026 | 4385             | 0.63991 | 0.926    |
|                     | 04/12/2029 | 5481             | 0.87609 | 0.87673  |
|                     | 04/12/2034 | 7307             | 1.19662 | 0.78698  |
|                     | 05/12/2039 | 9134             | 1.36455 | 0.71072  |
|                     | 05/12/2044 | 10961            | 1.45173 | 0.64665  |
|                     | 04/12/2054 | 14612            | 1.61238 | 0.52441  |
